# Supplementary material for: Cooperation and Fairness in Multi-Agent Reinforcement Learning
Source: arXiv:2410.14916 source file (2024-10-19)
Supplement: Supplementary file 1 [file 7_appendix.tex]

\appendix

\section{Appendix}
\label{sec:appendix1}
